# Supplementary material for: BotBuster: Multi-platform Bot Detection Using A Mixture of Experts
Source: arXiv:2207.13658 source file (2022-07-27)
Supplement: Supplementary file 1 [file appendix_doc.tex]

\relax
%File: formatting-instructions-latex-2022.tex
%release 2022.1
\documentclass[letterpaper]{article} % DO NOT CHANGE THIS
\usepackage{aaai22}  % DO NOT CHANGE THIS
\usepackage{times}  % DO NOT CHANGE THIS
\usepackage{helvet}  % DO NOT CHANGE THIS
\usepackage{courier}  % DO NOT CHANGE THIS
\usepackage[hyphens]{url}  % DO NOT CHANGE THIS
\usepackage{graphicx} % DO NOT CHANGE THIS
\urlstyle{rm} % DO NOT CHANGE THIS
  % DO NOT CHANGE THIS
\usepackage{natbib}  % DO NOT CHANGE THIS AND DO NOT ADD ANY OPTIONS TO IT
\usepackage{caption} % DO NOT CHANGE THIS AND DO NOT ADD ANY OPTIONS TO IT
\DeclareCaptionStyle{ruled}{labelfont=normalfont,labelsep=colon,strut=off} % DO NOT CHANGE THIS
\frenchspacing  % DO NOT CHANGE THIS
\setlength{\pdfpagewidth}{8.5in}  % DO NOT CHANGE THIS
\setlength{\pdfpageheight}{11in}  % DO NOT CHANGE THIS
%
% These are recommended to typeset algorithms but not required. See the subsubsection on algorithms. Remove them if you don't have algorithms in your paper.
\usepackage{algorithm}
\usepackage{algorithmic}

%%% REMOVE BEFORE SUBMISSION
\usepackage{xcolor}

%%% 
\usepackage{amsmath,amssymb,bm}
\usepackage{color, colortbl}
\definecolor{Gray}{gray}{0.9}
\usepackage{multicol}
\usepackage{lscape}

%
% These are are recommended to typeset listings but not required. See the subsubsection on listing. Remove this block if you don't have listings in your paper.
\usepackage{newfloat}
\usepackage{listings}
\lstset{%
	basicstyle={\footnotesize\ttfamily},% footnotesize acceptable for monospace
	numbers=left,numberstyle=\footnotesize,xleftmargin=2em,% show line numbers, remove this entire line if you don't want the numbers.
	aboveskip=0pt,belowskip=0pt,%
	showstringspaces=false,tabsize=2,breaklines=true}
\floatstyle{ruled}
\newfloat{listing}{tb}{lst}{}
\floatname{listing}{Listing}
%
%\nocopyright
%
% PDF Info Is REQUIRED.
% For /Title, write your title in Mixed Case.
% Don't use accents or commands. Retain the parentheses.
% For /Author, add all authors within the parentheses,
% separated by commas. No accents, special characters
% or commands are allowed.
% Keep the /TemplateVersion tag as is
\pdfinfo{
/Title (A Mixture of Experts Approach towards Social Bot Detection)
/Author (Lynnette Hui Xian Ng and Kathleen M. Carley)
/TemplateVersion (2022.1)
}

\setcounter{secnumdepth}{0} %May be changed to 1 or 2 if section numbers are desired.

% The file aaai22.sty is the style file for AAAI Press
% proceedings, working notes, and technical reports.
%

% Title

\title{A Mixture of Experts Approach towards Cross-Platform Social Bot Detection [Supplementary Information]}
\author{Anonymous Submission}
% \author{
%     Lynnette Hui Xian Ng\footnote{Corresponding Author}, Kathleen M. Carley\textsuperscript{\rm 1}
% }
% \affiliations{
%     \textsuperscript{\rm 1}CASOS, Institute for Software Research, \\ Carnegie Mellon University\\
%     \{huixiann,carley\}@andrew.cmu.edu
% }

\begin{document}

\maketitle

\input{appendix}

\newpage
\newpage
{\small
\bibliography{aaai22}}

\end{document}
